# Supplementary material for: CodeSift: An LLM-Based Reference-Less Framework for Automatic Code Validation
Source: arXiv:2408.15630 source file (2024-08-28)
Supplement: Supplementary file 1 [file appendix.tex]

\subsection{Single grading}
We assess the accuracy of single grading by utilizing LLMs as judges to evaluate the code quality score on a scale of 0 to 10. Subsequently, we establish thresholds ranging from 1 to 10 to derive binary judgments. If the assessed score equals or larger than the threshold, we classify the judge's assessment of the code as successful; otherwise, it is considered a failure. By comparing this binary judgment with runtime execution results, we calculate the accuracy, as illustrated in Table~\ref{tab:singlegrading}.

When Mistral is the judge, it performs more accurately on Llama2's generated code without any reference function.
For most of the cases, its judge accuracy decreases when reference functions are available except when it judges CodeLlama.

When Llama2 is the judge, it favors reference functions in the context. Its accuracy is notably higher when evaluating CodeLlama and code generated by itself.

\begin{table*}[t]
    \centering
     \caption{The single grading accuracy with different LLMs judging the generated code's quality. Each generation model generates results with and without reference functions.}
    \label{tab:singlegrading}
    \begin{tblr}{
        hline{1,11,Z}={1pt},
        hline{2}={solid},
        hline{odd}={solid},
        rows={m,rowsep=0pt,font=\footnotesize},
        colspec={X[c]|X[c]|X[-1,c]|X[-1,c]|X[-1,c]|X[-1,c]|X[-1,c]|X[-1,c]|X[-1,c]|X[-1,c]|X[-1,c]|X[-1,c]},
        cell{1}{3}={c=10}{c},
        cell{3,11}{1}={r=8}{m},
        cell{1}{1,2}={r=2}{m},
        cell{3,5,7,9,11,13,15,17}{2}={r=2}{m},
        cell{8}{3} = {m,bg=gray!20,fg=black},
        cell{10}{4,5,6,7,8,9,10,12} = {m,bg=gray!20,fg=black},
        cell{5}{10,11} = {m,bg=gray!20,fg=black},
        cell{17}{10,11,12} = {m,bg=gray!20,fg=black},
        cell{18}{12} = {m,bg=gray!20,fg=black},
        cell{11}{3,4,5,6,7} = {m,bg=gray!20,fg=black},
        cell{13}{8} = {m,bg=gray!20,fg=black},
        cell{17}{9} = {m,bg=gray!20,fg=black},
    }
    \textbf{Judge Model}	 &	\textbf{Gen. Model}	& \textbf{Threshold}	&&&&&&&&&\\    
             &  & 1    & 2    & 3    & 4    & 5    & 6    & 7    & 8    & 9    & 10\\
    Mistral & CodeLlama & 0.51 & 0.55 & 0.56 & 0.59 & 0.59 & 0.60 & 0.58 & 0.55 & 0.58 & 0.58\\
            &           & 0.48 & 0.47 & 0.46 & 0.47 & 0.48 & 0.48 & 0.48 & 0.50 & 0.51 & 0.56\\
            & StarCoder & 0.42 & 0.54 & 0.55 & 0.61 & 0.61 & 0.61 & 0.58 & 0.70 & 0.71 & 0.71\\
            &           & 0.34 & 0.34 & 0.34 & 0.38 & 0.38 & 0.38 & 0.39 & 0.46 & 0.54 & 0.64\\
            & Mistral   & 0.42 & 0.42 & 0.42 & 0.41 & 0.41 & 0.42 & 0.45 & 0.58 & 0.60 & 0.60\\ 
		&			& 0.54 & 0.58 & 0.57 & 0.59 & 0.60 & 0.59 & 0.59 & 0.60 & 0.61 & 0.61\\
            & Llama2    & 0.34 & 0.41 & 0.40 & 0.42 & 0.42 & 0.42 & 0.47 & 0.63 & 0.68 & 0.70\\ 
		&			& 0.49 & 0.63 & 0.62 & 0.66 & 0.66 & 0.66 & 0.66 & 0.70 & 0.70 & 0.73\\ 	
    Llama2  & CodeLlama & 0.50 & 0.50 & 0.53 & 0.55 & 0.56 & 0.54 & 0.56 & 0.63 & 0.52 & 0.52\\
            &           & 0.48 & 0.48 & 0.48 & 0.48 & 0.49 & 0.49 & 0.50 & 0.52 & 0.52 & 0.53\\
            & StarCoder & 0.35 & 0.36 & 0.47 & 0.50 & 0.55 & 0.55 & 0.62 & 0.72 & 0.68 & 0.69\\
            &           & 0.31 & 0.32 & 0.32 & 0.32 & 0.33 & 0.33 & 0.35 & 0.45 & 0.66 & 0.68\\
            & Mistral   & 0.39 & 0.41 & 0.42 & 0.44 & 0.45 & 0.47 & 0.55 & 0.63 & 0.63 & 0.63\\
            &           & 0.37 & 0.38 & 0.42 & 0.44 & 0.49 & 0.50 & 0.53 & 0.58 & 0.63 & 0.63\\ 
            & Llama2    & 0.32 & 0.34 & 0.40 & 0.42 & 0.48 & 0.52 & 0.64 & 0.73 & 0.75 & 0.75\\ 
		  &		      & 0.25 & 0.27 & 0.31 & 0.35 & 0.44 & 0.44 & 0.55 & 0.63 & 0.74 & 0.75\\ 

    \end{tblr}
\end{table*}
